# Supplementary material for: Biobeam - Rigorous wave-optical simulations of light-sheet microscopy
Source: arXiv:1706.02261 ancillary file (2017-06-09)
Supplement: Supplementary file 1 [file supplemental_notes_small.pdf]

# Supplementary Material

## Biobeam – Rigorous wave-optical simulations of light-sheet microscopy

Martin Weigert, Eugene W. Myers & Moritz Kreysing

May 11, 2017

## Supplementary Videos

**Video 1**: Wave-optical simulation of the image-formation process in light-sheet microscopy: The tissue model represents a multicellular (760 nuclei) organism of size $(100\mu m, 200\mu m, 100\mu m)$ in an aqueous medium with $n = 1.33$. The refractive index distribution is in the range $n \in (1.35, 1.42)$ comprising reference values for cell nuclei, eggshell and the cytoplasm[1]. Weak absorption is homogenously present, but could also be localized (e.g. a spherical absorbing compartment in the center). The simulations of both the illumination and detection processes were carried out on a computational grid of $(1024, 2048, 1024)$ voxels with a spacing of $100nm$ along each dimension. The illumination field is a cylindrical light sheet with $NA_{illum} = 0.1$ focused laterally at the center and the detection system was assumed to have $NA_{detect} = 0.6$. For generating the final stack both illumination and detection fields were simulated at 200 different axial positions. The deterioration of both resolution and intensity at regions where photons along either the illumination detection path had to travel through large inhomogeneities can clearly be seen.

**Video 2**: Illustration of *biobeam*'s detection PSF calculation process via propagation of diffraction limited fields.

**Video 3**: A *biobeam* generated video illustrating rigorous wave-optical mimicry of a wide-field microscope. Imaging of a $100\mu m^2$ test chart is simulated while a strongly aberrating refractive index heterogeneity is continuously introduced into the microscope's optical path.

**Video 4**: Screencast of an interactive command line session demonstrating *biobeam*'s capabilities and speed. All calculations happen in real time.

**Video 5**: Video showing the predefined illumination modes and simulated light sheets being scanned through a biological plausible tissue model. Both coherent (cylindrical

lens SPIM) illumination and partially-incoherent illumination modes (time scanned Gaussian/Bessel beams) are simulated.

**Video 6**: Showing the simulation of a aberration pre-compensated wavefront focusing deep into tissue and the shift-shift memory effect.

**Video 7**: Example of a plane-by-plane illumination of a tissue model mimicking an embryo.

# Supplementary Figures

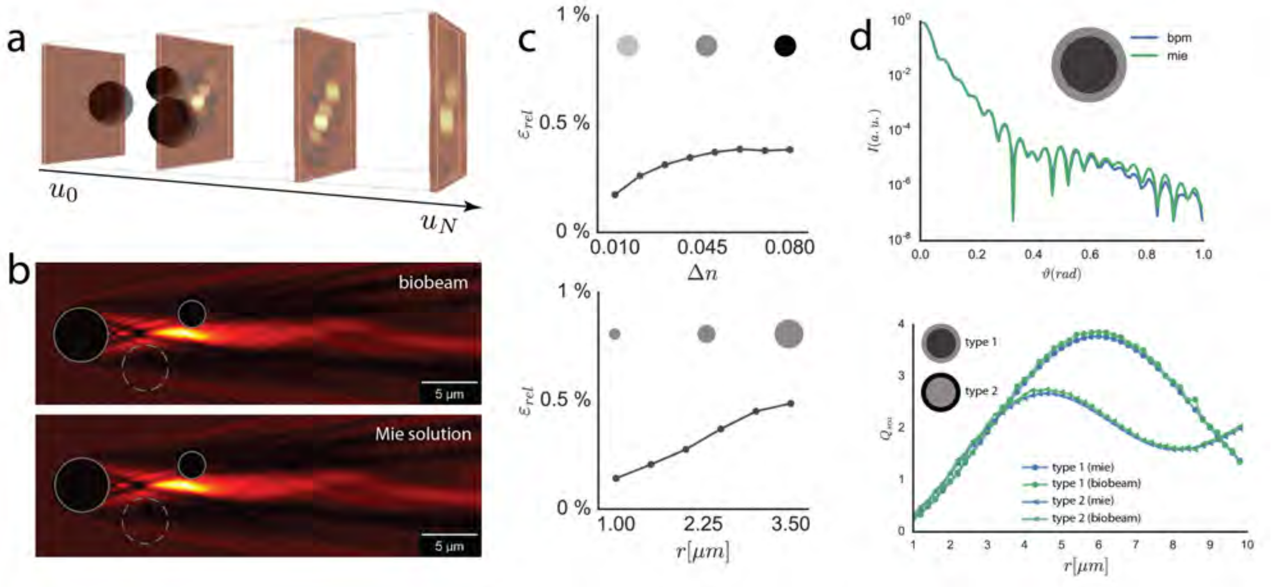


**Supplementary Figure 1:** Validation of *biobeam* with analytical solutions. a) Plane wave scattered by three solid spheres ($\lambda$=500$nm$, r=2-2.5$\mu m$, refractive index contrast m=1.05), b) Comparison of analytical solution (Mie calculus) versus *biobeam* simulation. c) Error percentage of near field distribution as a function of single sphere radius r ($\Delta n$ = 0.05) and refractive index contrast $\Delta n$ (r=2.5$\mu m$). d) Left: Phase function of analytically tractable coated spheres as cell models (m=1.02/1.04, r=5$\mu m$/4$\mu m$) shows high accuracy up to approximately 0.5 radians. Right: size dependent scattering efficiency of the same sphere architecture and its inverse.

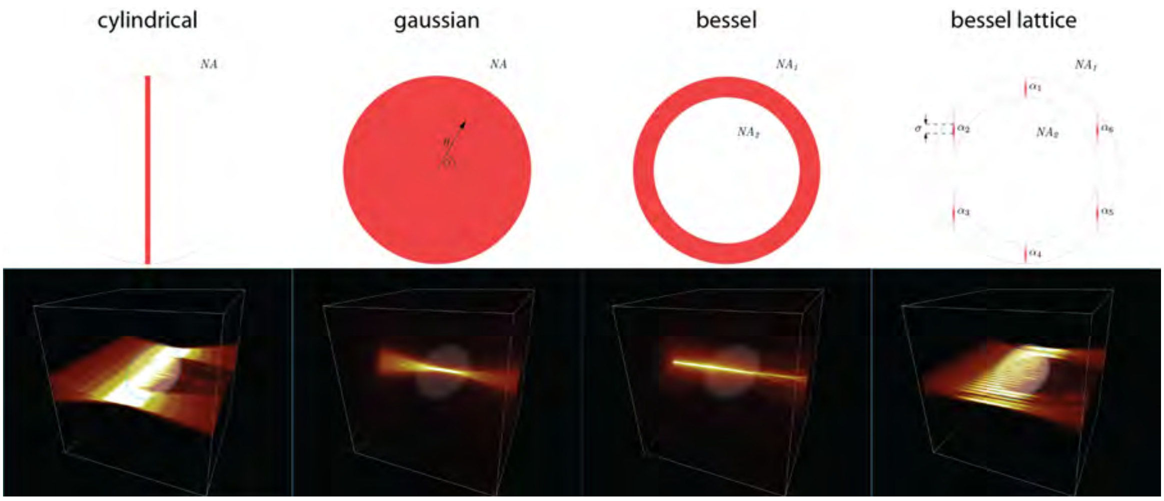


**Supplementary Figure 2:** Propagation of different predefined input fields through a tissue model of size $(100\mu, 100\mu, 100\mu)$ and grid dimension $(1024^3)$. The respective pupil function is shown in the upper row.

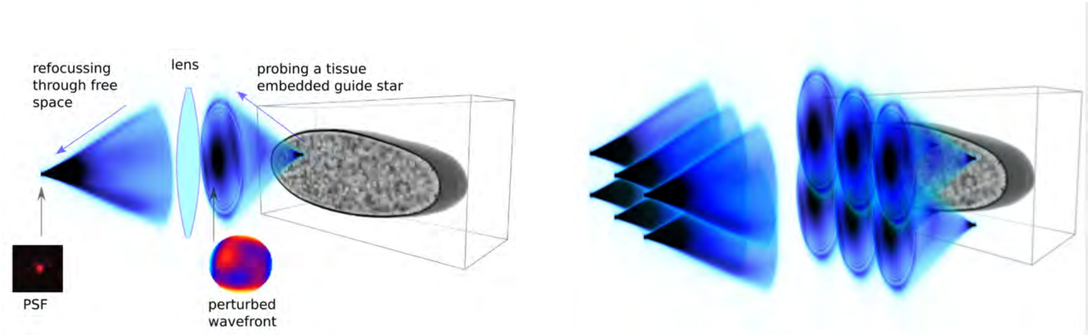


**Supplementary Figure 3:** Detection aberration and PSF calculation. Propagating a diffraction limited input field through parts of the sample and refocusing by an idealized optical system gives the focus field as seen by the detector. If the refocus spots are separated for different starting points, the propagation of a complete grid can be carried out in a highly multiplexed manner, accelerating the process for typical microscopy simulations by a factor 100–1000.

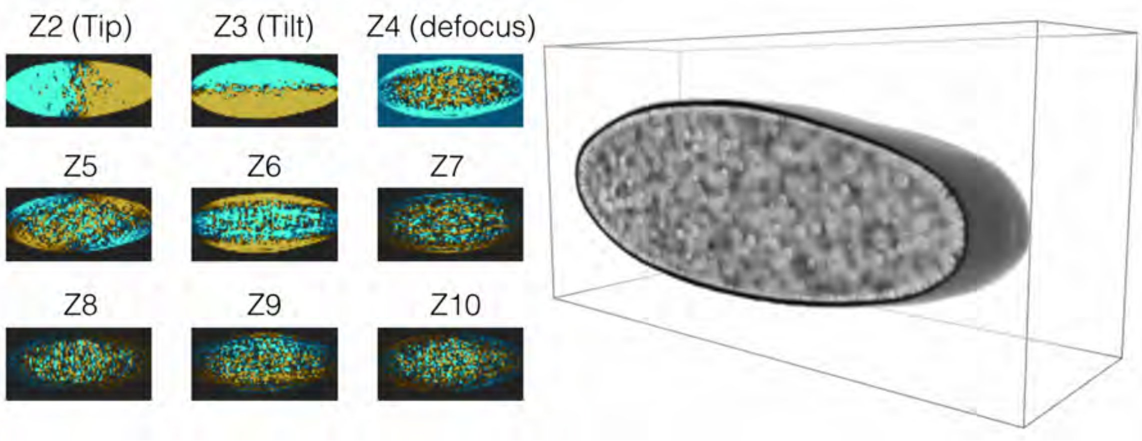


**Supplementary Figure 4:** Calculating the aberrations of the detection point spread function (PSF) for a given z plane within a synthetic tissue model. The model's physical size is $(200\mu m, 100\mu m, 100\mu m)$ and the dimension of the computational grid are $(1024, 512, 512)$. The detection wavelength is $\lambda = 522nm$, the numerical aperture is $NA = 0.5$ and the aqueous immersion medium has refractive index $n_0 = 1.33$. The refractive index distribution of the tissue model mimics an eggshell, cell nuclei and granular random fluctuations within the biological plausible range of $n \in (1.35, 1.43)$.

# Supplementary Notes

1 Numerical methods 4

2 Software implementation & practical use of *biobeam* 6

3 Examples of *biobeam* programs 8

4 Validation 11

5 Performance and comparison with existing software 12

6 Wave optical forward model in light-sheet microscopy 13

7 Image-formation in light-sheet microscopy 14

8 PSF calculations, single and multiplexed 15

9 Multiplexed aberration calculations 16

10 Details of memory effect simulations 17

## 1 Numerical methods

At the lowest level *biobeam* currently uses the well described scalar beam propagation method (BPM [2, 3]) along with locally reduced refractive index contrasts and a mathematically exact propagator which's use we explain and justify in the following:

The simulation of light propagation through tissue amounts to solving for the electrical field $\vec{E}(x, y, z)$ given a refractive index distribution $n(x, y, z)$ and certain boundary conditions. This in general requires the numerical treatment of the time dependent vectorial *Maxwell's equations*[4]. For monochromatic illumination along $z$ and low refractive index differences however, a far simpler description in terms of a complex scalar field $u(x, y, z)$ becomes applicable, and the problem reduces to solving the scalar *Helmholtz equation*[4]:

$$\Delta u(\mathbf{r}) + n(\mathbf{r})^2 k_0^2 u(\mathbf{r}) = 0, \qquad k_0 = \frac{2\pi}{\lambda} \tag{1.1}$$

This approximation exploits the fact that refractive index variations in biological cells are small and light scattering in tissues is predominantly forward directed [5, 6], and that forward directed light scattering determines imaging aberrations. Although thereby back-scattering of light on the way from the specimen to the lens is neglected, this is justified for simulation of the image formation process in tissues, as *i)* this light would only contribute to the final image when changing direction a second time, *ii)* also adaptive optics aberration correction requires the forward scattered photons only.

Eq. (1.1) can be now solved in the spectral or angular spectrum domain [7] by propagating the field $u(x, y, z)$ at position $z$ to $z + \Delta z$ via

$$u(x, y, z + \Delta z) = \int dk_x dk_y \mathcal{F}[u] H(x, y, z, k_x, k_y) e^{i(k_x x + k_y y)} \tag{1.2}$$

where $\mathcal{F}[u](x, y, z) = \int dk_x dk_y u(k_x, k_y, z) e^{-i(k_x x + k_y y)}$ is the 2D Fourier transform of $u$ and $H = e^{i\Delta z \sqrt{n(x,y,z)^2 k_0^2 - k_x^2 - k_y^2}}$ is the accurate (i.e. non paraxial) propagator in the Fourier domain. In a further approximation the refractive index is assumed to be a small variation around a constant $n(x, y, z) = n_0(z) + \Delta n(x, y, z)$ so that the final approximation gives the scalar beam propagation

$$u(x, y, z + \Delta z) \approx \mathcal{F}^{-1}\left[\mathcal{F}[u(x, y, z)] e^{i\Delta z \sqrt{n_0(z)^2 k_0^2 - k_x^2 - k_y^2}}\right] e^{i\Delta z \Delta n k_0} \tag{1.3}$$

which can be efficiently solved by operator split stepping via FFTs and point wise multiplications [2, 3].

To simulate the actual light propagation, we first assume the tissue to be given by a complex grid of refractive indices n(r) after which we employ the classical scalar Fourier transform beam propagation method (FFT-BPM [3]) which solves the scalar Helmholtz equation by a operator split stepping, i.e. first freely propagating the complex field on a given z-plane and then multiplying it by the complex phase difference of the tissue.

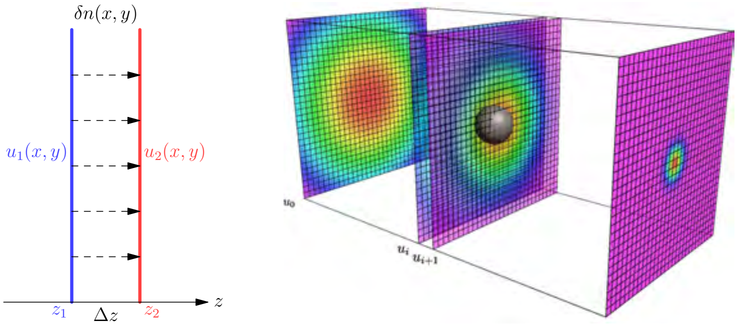


**Figure 1:** Principle of beam propagation: each $z$-plane is first propagated freely and then a space dependent phase shift is multiplied.

Crucial for the performance of BPM is a good choice of the refractive index representation $n_0(z)$ while propagating the fields because BPM otherwise quickly become inaccurate for non-paraxial light fields. The problems one may encounter here is twofold. i) Phase shifts at large angles are underrepresented when refractive index contrasts are high, since the increasing path length with angle is not represented. ii) Inaccuracy could of course also be introduced in the propagator if the implementation does not match

the refractive index representation to calculate phase shifts. To minimize inaccuracies for at high angles in regions of large refractive index contrasts, the following representations increase accuracy stepwise:

(a) constant: sets $n_0 = \text{const}$, typically $n_0 = \langle n \rangle_{x,y,z}$, i.e. to the full average of $n$. This reduces the average refractive index of tissues from typical values 1.37 to 1, thus the remaining refractive index contrast to deal with are just the relative variations that occur in a tissue, typically on the order of +- 0.03 %.

(b) full average: sets $n_0(z) = \langle n \rangle_{x,y}$, i.e. to the per-plane average of $n$. This bears two advantages. 1) It effectively allows the modeling of aberrations that occur at planar interfaces of high refractive index contrast, i.e. a cover glass or implications of a mismatched working distance. 2) Biological tissues often possess a planar stratification, which implies plane wise varying average refractive indices that can be dealt with more efficiently.

(c) weighted average: sets $n_0(z) = \langle |u|n \rangle_{x,y} / \langle |u| \rangle_{x,y}$, i.e. to the per-plane average weighted by the field magnitude. This choice is even better since additionally to stratification averages, accounts also for finite lateral dimensions of samples like embryos, i.e. the refractive index for the calculation of the average is only taken into account when the light field is factually overlapping with it.

Already the 1st strategy quoted here largely reduces the problem of inaccuracy of phase projections of high refractive indices at large angles. The two additional tweaks are not generally applicable to any physical light scattering problem, but are significant practical relevance when dealing with biological samples.

Furthermore each algorithmic step is executable in a parallel fashion this method is therefore highly receptive to the parallelization by architecture of modern Graphic Processor units (GPUs). It can be used to calculate the propagation of light through any low contrast refractive index distribution. By this *biobeam* leverages on the enhanced computing power of modern GPUs and attain a significant performance gain compared to a pure CPU implementation (see Section 3).

## 2 Software implementation & practical use of *biobeam*

The method was implemented within the open source Python[1] software package *biobeam* using OpenCL[2] as the GPU programming architecture. As the computationally heavy parts are lifted to the GPU, we thereby keeping all the advantages of Python as a dynamically typed high level language that is vastly used in the scientific community without compromising on performance. We chose OpenCL for its availability on all major GPU platforms (NVIDIA, AMD, Intel) and use the excellent Python bindings provided by PyOpenCL[3][8]. We further make use of our own utility libraries gputools[4] (for GPU based FFTs, fast spatially varying convolutions, etc) and *spimagine*[5] (rendering/visualization).

[1] Python Software Foundation, http://python.org
[2] Khronos Group, http://khronos.org/opencl
[3] `https://documen.tician.de/pyopencl/`
[4] `https://maweigert.github.io/gputools/`
[5] `https://maweigert.github.io/spimagine/`

Apart from its technical focus on speed, *biobeam* was specifically designed to make wave optical experiments in-silico as easy as possible. As an example, the listing 2 shows how to propagate a Bessel beam with the annulus defined by the apertures $NA_1 = 0.4, NA_2 = 0.43$ and focal point $50\mu m$ through a random refractive index volume (n $= 1.33 \pm 0.05$) of size $(100\mu m)^3$ on a grid volume $(512, 512, 512)$ and returning the complete complex field on the grid.

*biobeam*'s API further makes it easy to apply different input fields as well as PSF/aberration calculations by propagating diffraction limited point sources from within the tissue. Examples and detailed documentations can be found on at https://maweigert.github.io/biobeam/.

**Input fields** *Biobeam* offers the possibility to define input fields not only according to the Fourier transform of the aperture function $P(\theta, \phi)$, but more accurately according to the vectorial Debye-Wolf integral (just the x component is shown for brevity, see [9]):

$$E_x(\rho, \varphi, z) = -\frac{ikfE_x^0}{4\pi} \int_0^\alpha \int_0^{2\pi} d\theta d\phi\, P(\theta, \phi) \sqrt{\cos\theta} \sin\theta \left[ (\cos\theta + 1) + (\cos\theta - 1) \cos 2\phi \right] \cdot e^{ik\rho \sin\theta \cos(\phi - \varphi)} e^{ikz\cos\theta} \tag{2.1}$$

| Cylindrical sheet | Gaussian beam | Bessel beam | Bessel Lattice [10] |
|---|---|---|---|
| `u0_cylindrical(NA=.3)` | `u0_beam(NA=.6)` | `u0_beam(NA=(.3,.32))` | `u0_lattice()` |

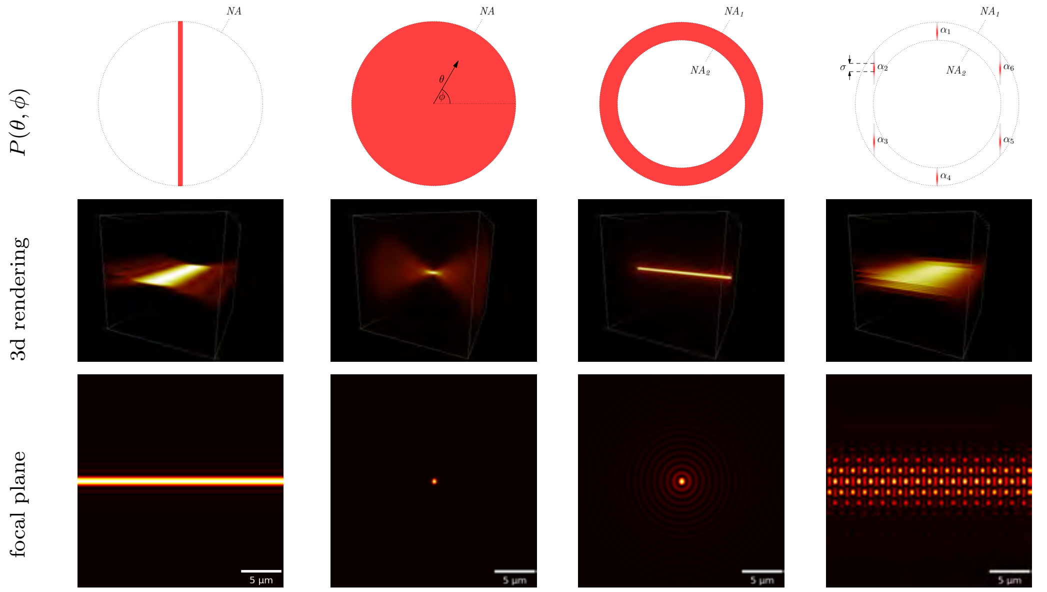


**Table 1:** Different pupil functions and the resulting focus fields as generated by *biobeam*

*Biobeam* uses the correctly calculated $E_x$ as input field for the different illumination modes. For that reason the package implements the fast GPU based calculation of these types of volumetric diffraction integrals and PSFs. See listing 1 for a simple example for a Bessel beam.

## 3 Examples of *biobeam* programs

In this section we give some explicit examples how easy it is to set up wave optical simulations with *biobeam*.

**Listing 1:** Focussing a Gaussian beam in free space

```
from biobeam import focus_field_beam

# a Gaussian beam with NA = 0.4
intensity = focus_field_beam(
                   shape = (256,256,256),
                   units = (0.1,0.1, 0.1),
                   NA = 0.4)
```

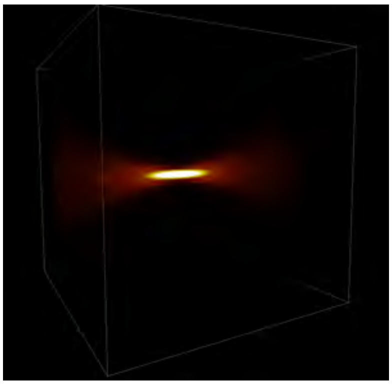

**Listing 2:** Propagation of a Bessel beam through a tissue phantom, which is given by a Perlin noise refractive index distribution

```
from biobeam import Bpm3d
from gputools import perlin3

# set up the refractive index distribution
dn  = 0.03*perlin3((512,512,512),scale = 4)

# set up the propagator class
m = Bpm3d(dn = dn, size = (70,70,70),
          lam = .5,n0 = 1.33)
# propagate the light field...
field = m.propagate(u0 =
            m.u0_beam(NA = (0.4,.41)))
```

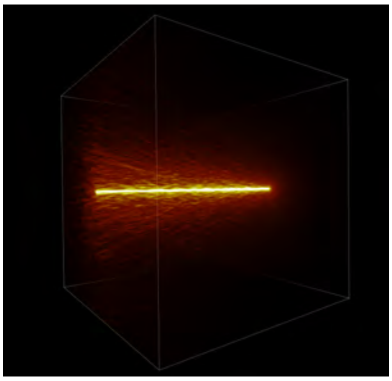

**Listing 3:** Calculation of the spatially varying PSFs at a plane inside of a refractive sphere

```
import numpy as np
from biobeam import SimLSM_Cylindrical

def create_dn(N = 512):
        """generates a refractive sphere"""
    x = np.linspace(-50,50,N)
    Xs = np.meshgrid(x,x,x,indexing = "ij")
    R = np.sqrt(np.sum([_X**2 for _X in Xs],
        axis = 0))
    #generate the refractive index differences
    dn = .04*(R<20)
    return dn

dn = create_dn()

#create a microscope simulator
m = SimLSM_Cylindrical(dn=dn,
                NA_illum=.1,NA_detect=.6,
                size = (100,100,100), n0 = 1.33)

# simulate the psf grid at an axial position
# -20um relative to center
psfs = m.psf_grid_z(cz=-20, grid_dim=(16,16),
                        with_sheet = False)
```

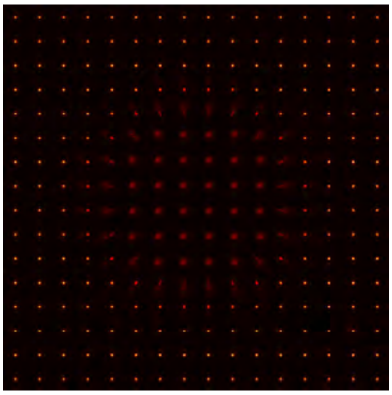

**Listing 4:** Simulating the image formation of a light-sheet microscope in the presence of a tissue phantom represented by a inhomogeneous refractive sphere of $70\mu m$ diameter. Light sheet in image plane is entering from the left. Time to run should be less than 5 seconds.

```
import numpy as np
from biobeam import SimLSM_Cylindrical
from biobeam.data import tiling
from gputools import perlin3

def create_dn_and_signal(N = 512):
    """generates a refractive inhomogeneous
    sphere and an image as given by the
    function tiling()"""
    x = np.linspace(-50,50,N)
    Xs = np.meshgrid(x,x,x,indexing = "ij")
    R = np.sqrt(np.sum([_X**2 for _X in Xs],
                          axis = 0))
    #generate the refractive index differences
    dn = (.07+0.02*perlin3((N,N,N), scale =3))\
                          *(R<35)
    #replace call to tiling() with own image
    signal = np.einsum("i,jk",np.ones(N),
                          tiling(N))
    return dn, signal

dn, signal = create_dn_and_signal()

#create a microscope simulator
m = SimLSM_Cylindrical(dn=dn, signal=signal,
                NA_illum=.1, NA_detect=.45,
                size = (100,100,100), n0=1.33)

# generate image as recorded by the microscope
# at an axial position -20um relative to center
image = m.simulate_image_z(cz=-20,
psf_grid_dim=(16,16),conv_sub_blocks=(2,2))[16]
```

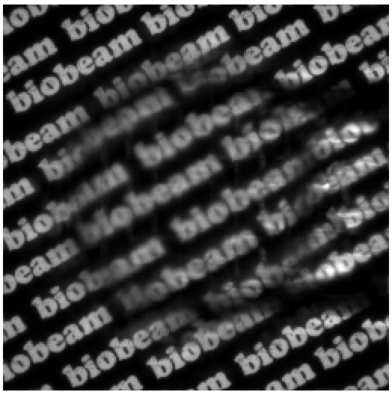

**Listing 5:** Simulating a light-sheet passing through a refractive sample

```
from biobeam import SimLSM_Cylindrical

#create some input data, r.i and labeled density
dn, signal = generate_some_refractive_volume_and_label()

#create a microscope simulator
m = SimLSM_Cylindrical(dn = dn, signal = signal,
                          NA_illum= .1, NA_detect=.6,
                          size = size, n0 = 1.33)
```

```python

#simulate the image at relative  axial position 20um
image = m.simulate_image_z(cz=20)
```

**Listing 6:** Calculating the psf grid at a specific axial position

```python
from biobeam import SimLSM_Cylindrical

#create some input data, r.i and labeled density
dn, signal = generate_some_refractive_volume_and_label()

#create a microscope simulator
m = SimLSM_Cylindrical(dn = dn, signal = signal,
                       NA_illum= .2, NA_detect=.6,
                       size = size, n0 = 1.33)

#simulate the image at realtive axial position 20um
psfs = m.psf_grid_z(cz=20, grid_dim=(32,32))
```

# 4 Validation

To validate the accuracy of the described BMP implementation we compared numerically obtained field distributions with analytically tractable models. Specifically we analyzed the case of incident plane wave scattered by spheres of diameter $5\mu m$ and with a refractive index contrast of 5% as calculated by *biobeam* with the precise mathematical solution (calculated with the Mie code GMMFIELD[6][11] ).

We further calculate the scattering phase function $f(\theta, \phi)$ and scattering cross section $\sigma$ from the angular spectrum $\tilde{U}(k_x, k_y, z_{last})$ of the last plane via

$$\begin{aligned} f(\theta,\phi) &= -ik_0\cos\theta\tilde{U}(k_0\cos\phi\sin\theta, k_0\sin\phi\sin\theta) \\ \sigma &= \int dk_x dk_y |\tilde{U}(k_x,k_y)|^2\sqrt{1-k_x^2/k_0^2-k_y^2/k_0^2} \end{aligned} \tag{4.1}$$

For a concentrically coated sphere as an analytically tractable cell model, with a cytoplasmic fraction and higher refractive cell nucleus, the results are near identical (Supp. Fig. 1 c) in both near and far field. Significant relative errors only arise at high angles (see phase function comparison in Supp. Fig. 1d upper graph) at which however little intensity is scattered. We further calculated the scattering efficiencies for coated spheres with various size parameters and compared them to analytical results showing good agreement (see scattering efficiency comparison in Supp. Fig. 1d lower graph). Relative field errors in the analytically limiting case of 3 spheres are still below 1% evaluated over the near-field over a $35\mu m$ big computational cell and all angles (refractive index contrast 3%).

[6] http://moritz-ringler.name/dissertation/GMM_FIELD.tar.bz2

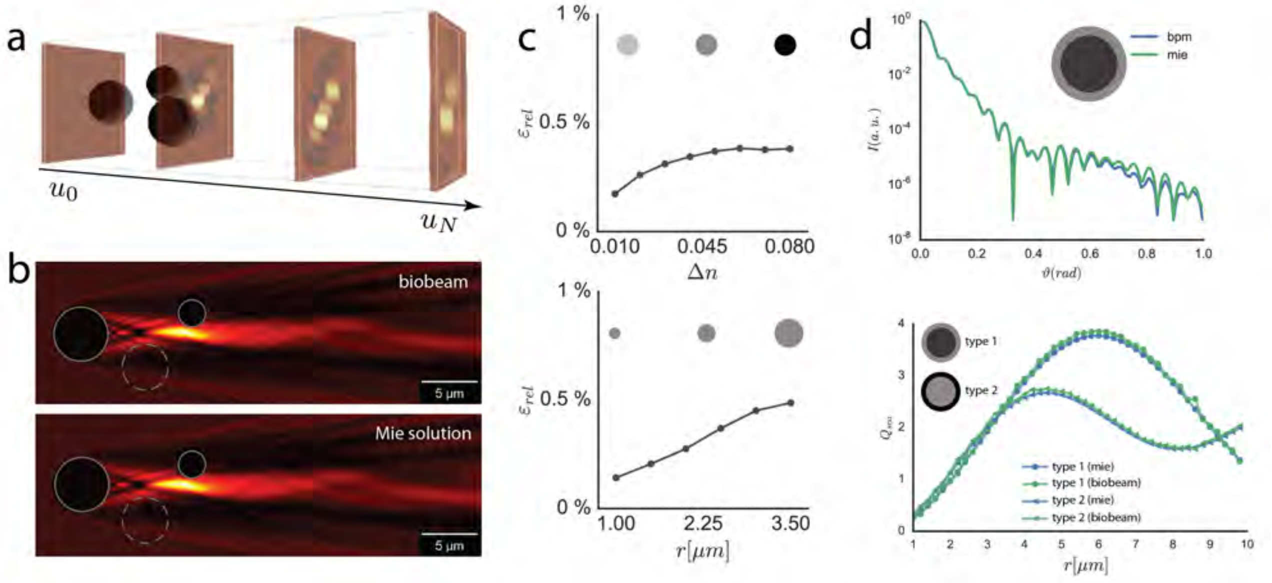


**Figure 2:** Validation of *biobeam* with analytical solutions. a) Plane wave scattered by three solid spheres ($\lambda$=500$nm$, r=2-2.5$\mu m$, refractive index contrast m=1.05), b) Comparison of analytical solution (Mie calculus) versus *biobeam* simulation. c) Error percentage of near field distribution as a function of single sphere radius r ($\Delta n$ = 0.05) and refractive index contrast $\Delta n$ (r=2.5$\mu m$). d) Top: Phase function of analytically tractable coated spheres as cell models (m=1.02/1.04, r=5$\mu m$/4$\mu m$) shows high accuracy up to approximately 0.5 radians. bottom: size dependent scattering efficiency of the same sphere architecture and its inverse.

## 5 Performance and comparison with existing software

We compareed the attainable performance of *biobeam* with available open source programs, specifically with MEEP[12][7], which implements the Finite Difference Time Domain (FDTD) method to solve Maxwells' equation and the Mie code GMMFIELD[11] for internal field calculations.

| Dimension ($x \times y \times z$ ) | Mie code (GMMFIELD) | FDTD (MEEP) | *biobeam* BPM |
|---|---|---|---|
| (128,128,128) | 1314s | 80 s | 34 ms |
| (256,256,256) | 10480s | 790 s | 81 ms |
| (512,512,512) | – | 4800 s | 154 ms |
| (1024,1024,1024) | – | – | 440 ms |

**Table 2:** Runtimes of plane wave propagation through a given refractive index distribution of given dimensions

The runtime differences of several orders of magnitude clearly demonstrates the superiority of the BPM as implemented on GPUs. This efficiency results a scaling of operations directly proportional to the penetration depth into the tissue compared to Mie and FDTD codes, and a further speed up due to the massively parallelization of remaining operations on the GPU.

[7] http://ab-initio.mit.edu/wiki/index.php/Meep

To measure the speedup of the GPU/OpenCL based implementation compared to a pure CPU (in C) and GPU/CUDA implementation we compared the runtime of a plane wave propagating through a constant refractive index distribution for three different basic implementations of the BPM method.

**CPU** Single precision implementation in C (FFTW 3.3 with `FFTW_MEASURE` as FFT library), and different levels of multithreading with 1, 4 or 16 threads (*red, ochre, green*)

**GPU1** Python with PyCuda bindings, (*cyan*)

**GPU2** Python with PyOpenCL bindings, (*purple*)

The hardware used was a 20 core Xeon(R) CPU E5-2660 v3 (2.60GHz, 64GB RAM) workstation for the CPU benchmarks, and a NVIDIA GeForce GTX Titan X (12GB RAM) for the GPU ones.

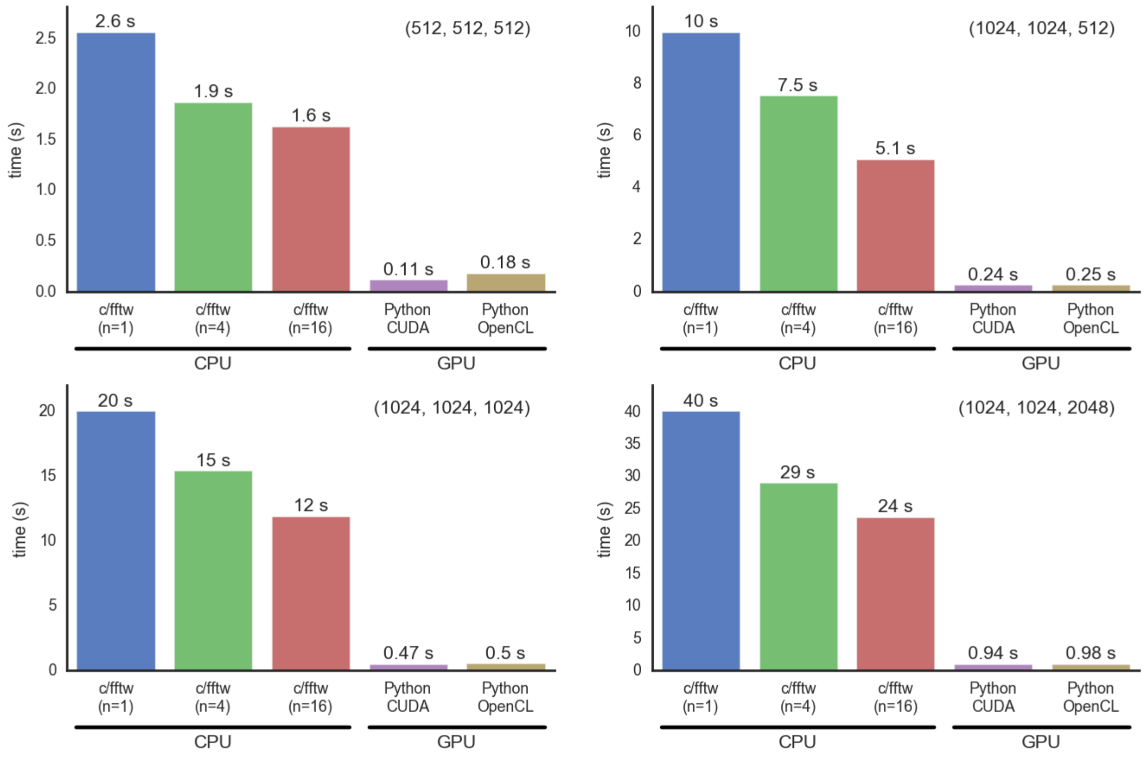


**Figure 3:** Comparison for different BPM implementations on CPU vs GPU

The performance of both the OpenCL and CUDA implementation are compareable and the overall speedup when of the OpenCL version compared to the single threaded CPU version was between 15–40 and to the 16-multithreaded version between 10–25, where the greater speedups were achieved in the relevant scenario of bigger propagation volumes.

## 6 Wave optical forward model in light-sheet microscopy

*Biobeam* is modular software suite to enable the simulation of the image formation process in tissue microscopy. While the modularity of our software enables to flexibly implement the simulation of different imaging modalities, we exemplify *biobeam* performance by the implementation of a light-sheet microscope, which makes use of two distinct light paths, one for excitation and one for the collection

of fluorescent light. We start this section with a general description of the process and complement this by the detailed explanation of how *biobeam* efficiently carries out the actual simulations required to faithfully mimic the microscopy process.

## 7 Image-formation in light-sheet microscopy

Light-sheet microscopy achieves optical sectioning by the orthogonality between the illumination and the detection axis [13]. To model the image-formation process let

$f(x, y, z)$ , the fluorophore density in the sample
$h(x, y, z)$ , the PSF of the detection objective
$j(x, y, z)$ , the illumination intensity (PSF) of the light sheet
$g(x, y, z)$ , the observed volumetric intensity (image)

where $z$ is the coordinate along the optical axis of the detection objective and $y$ the propagation axis of the illuminating field. Let the current focal position be $z_F$ and fixed. Then the excited intensity distribution of the fluorophore $\tilde{f}(x, y, z)$ is

$$\tilde{f}(x, y, z) = f(x, y, z) \cdot j(x, y, z_F - z) \tag{7.1}$$

For each constant slice at $z$ the intensity $\tilde{f}(x, y, z)$ gets convolved with $h(x, y, z_F - z)$ resulting in

$$\begin{aligned} a(x, y, z_F, z) &= \int dx'dy'h(x', y', z_F - z)\tilde{f}(x - x', y - y', z) && (7.2) \\ &= \int dx'dy'h(x', y', z_F - z)f(x - x', y - y', z)j(x - x', y - y', z_F - z) && (7.3) \end{aligned}$$

and the overall observed image plane $g(x, y, z_F)$ for a fixed focal position is then the integral of all contributions

$$g(x, y, z_F) = \int dx'dy'dz'h(x', y', z')f(x - x', y - y', z_F - z')j(x - x', y - y', z') \tag{7.4}$$

Note that if the illumination field can be factored as $j(x, y, z) = j_{xy}(x, y) \cdot j_z(z)$, then

$$g(x, y, z_F) = (h \cdot j_z) \otimes (f \cdot j_{xy}) \tag{7.5}$$

and the observed image $g$ is simply the 3 dimensional convolution of the illuminated density $f \cdot j_{xy}$ with an effective PSF $h_{eff} = h \cdot j_z$. For a distorted illumination field, this however is not true in general and the detection PSF as well typically varies spatially due to the distortions induced by the tissue. For modeling this complete image-formation process *biobeam* executes the following steps at every desired axial position $z_F$ (cf. Video 2):

1. computing the distorted illumination field $j$ at a given position $z_F$
2. calculating a fine grid of multiplexed spatially varying detection PSFs at that axial position, and

3. performing with it a spatially varying convolution of the product of the fluorophore signal and the 3d excitation profile to produce the final image at $z_F$ as seen by the detector.

For 1. the resulting PSFs are interpolated between sampling points to result in a quasi-continuum that can be used for an accurate convolution with a spatially varying, wave-optically determined kernel. The latter step is carried out based on standard methods [14]. The API of *biobeam* allows for a simple way of doing these image-formation simulations, as demonstrated by the listing 4 for the case of a cylindrical light-sheet microscope:

## 8 PSF calculations, single and multiplexed

**Single PSF** Point spread functions inside tissues were calculated by propagating light from tissue embedded, diffraction-limited airy disks corresponding to the given numerical aperture (NA) of the detection system towards an idealized lens. Here the resulting complex wave field is phase-conjugated and propagated back towards a focus, but this time through free space (cf. Video 2). For light-sheet microscopy simulations these point spread function are significantly further constrained in axial direction due to the small width of the independently simulated light sheet.

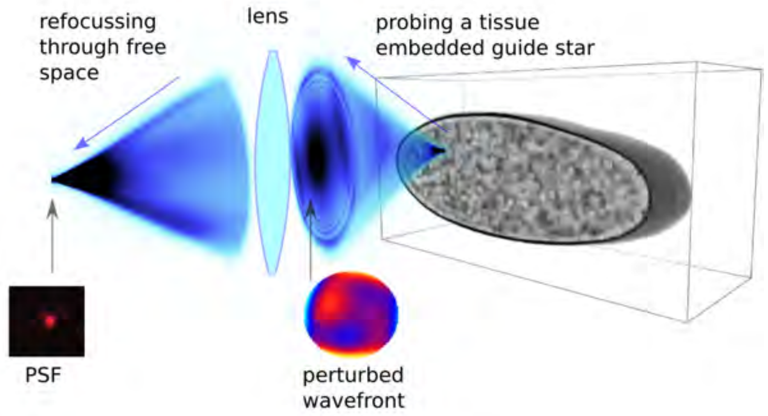


**Figure 4:** Single PSF calculation. Propagating a diffraction limited input field through parts of the sample and refocusing by an idealized optical system gives the focus field as seen by the detector

**Multiplexed PSFs** For the parallel simulation of a complete grid of spatially varying PSFs we exploit the fact that optics is linear, and sufficiently spaced point spread functions in a plane do not significantly overlap, hence can be propagated and refocused in multiplexed way (cf. Fig. 5). The PSF grid sampling is practically done at a grid-spacing below the smallest isoplanatic patch size in the sample, which are found at the most distant positions from the imaging lens, resulting in a sub-sampling of the volume proportional to the half-width of the aberration-autocorrelation function for the plane furthest from the objective. These PSFs are efficiently generated all at once in a multiplexed manner, i.e. a sub-grid of initial diffraction limited focal spots is propagated simultaneously through the volume and refocused together while ensuring that no substantial coherent overlap arises between neighboring PSFs (cf. Fig. 5 and Video 3). This reduces the computational complexity by the number of simultaneously calculated PSFs, i.e. typically 100-1000 fold.

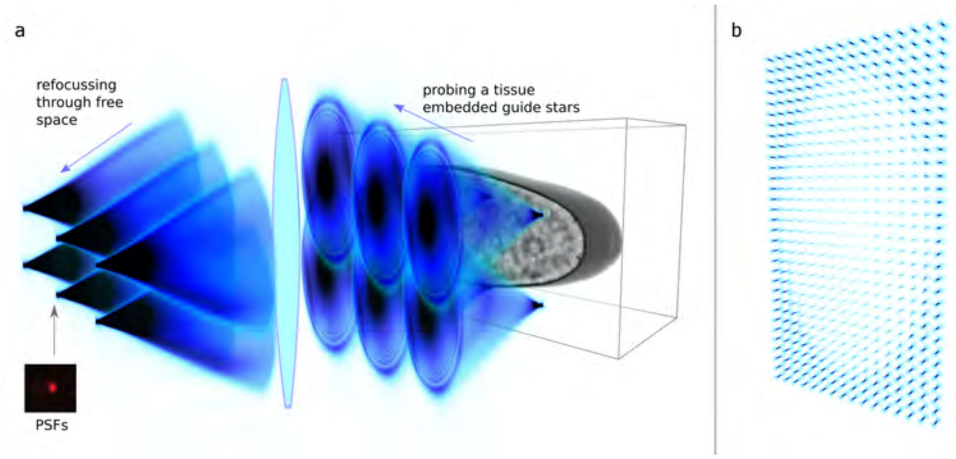


**Figure 5:** Multiplexed PSF calculation. a) If the refocus spots are separated for different starting points, the propagation of a complete grid can be carried out in a highly multiplexed manner, accelerating the process for typical microscopy simulations by a factor 100–1000. b) Grid of 16x32=512 PSFs calculated in a single simulation instance.

Listing 3 demonstrates how one can calculate the grid of point spread function in a highly multiplexed manner on a $(32 \times 32)$ grid at relative axial position $20\mu$ for a cylindrical lens SPIM with illumination $NA_{illum} = 0.2$ and detection $NA_{detect} = 0.5$.

# 9 Multiplexed aberration calculations

In practice, it might often be desired not only simulate sets of PSFs distributed over a sample, but to directly extract spatial maps of aberrations that would result when imaging a tissue or embryo that is represented in a refractive index model.

Given the efficiently multiplexed determination of PSF as described in the previous section (Fig. 5), also aberrations terms can efficiently be calculated for any point in a sample in the same manner. The main benefit again is that a single multiplexed simulation through the tissue is sufficient. Let $h(x-x_0, y-y_0, z_F)$ be the lateral slice of the PSF associated to a given initial position $(x_0, y_0)$ at focal position $z_F$, then the corresponding pupil function $P(\theta, \phi)$ is given by the properly rescaled Fourier transform of $h(x-x_0, y-y_0, z_F)$. Projecting $P(\theta, \phi)$ onto a Zernike basis yields the associated Zernike terms of the aberrations present at $(x_0, y_0, z_F)$. Fig. 6 shows a demonstration of these aberration calculations for a tissue model with a biological plausible refractive index distribution mimicking cell nuclei, cytoplasm and the eggshell of of $n \in (1.35, 1.43)$ [1].

*Biobeam* is highly efficient in determining sample induced aberration for given refractive index models (cf. Fig. 6). For this, light from diffraction limited guide-stars is propagated to the back-pupil of a virtual microscope. Recorded field can then be composed according to Zernike aberration modes. For this we record the complex scalar product between the field distribution and each Zernike mode on a pupil representing unit-sphere (see ref 2).

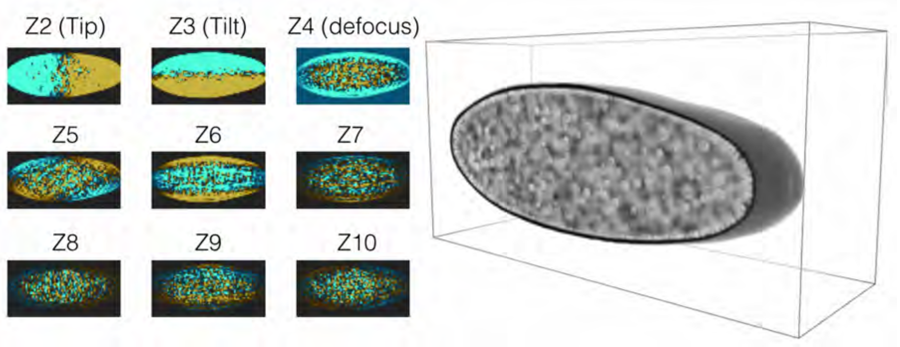


**Figure 6:** Calculating of Zernike aberration terms for the detection point spread functions (PSF) at a given z plane within a synthetic tissue model. The model's physical size is ($200\mu m$, $100\mu m$, $100\mu m$) and the dimension of the computational grid are $(1024, 512, 512)$. The detection wavelength is $\lambda = 522nm$, the numerical aperture is $NA = 0.5$ and the aqueous immersion medium has refractive index $n_0 = 1.33$. The refractive index distribution of the tissue model mimics an eggshell, cell nuclei and granular random fluctuations within the biological plausible range of $n \in (1.35, 1.43)$.

# 10 Details of memory effect simulations

The shift-shift memory effect [5] describes the behavior of an aberration corrected and therefore diffraction limited focal spot when laterally translated within a scattering tissue. Given a fixed position $g$, such focus can be created by pre-shaping the incoming wavefront with the correct wavefront aberration terms $\phi_g$ [15]. When translated laterally by a length $\Delta x$, the quality of the resulting spot at the translated position quickly deteriorates (Video 6), albeit in a charactized manner: The correlation coefficient as a function of $\Delta x$ between the original and the laterally shifted focal spot is equal the autocorrelation function of the speckle pattern resulting from an incident plane wave at the same depth [5].

To simulate the memory effect as in Fig. 1, we first created synthetic refractive index distributions of different depth ($N_x/N_y = 100\mu m, N_z = 20 \ldots 80\mu m$) and with refractive index variation of $n = 1.35 \pm 0.03$ by either randomly placing hard spheres in the volume or using generated Perlin noise of the given variation. Next, diffraction limited guide stars were implemented inside this tissue dummy and propagated to its surface, where the guide-star specific aberration patterns $\phi_g$ were recorded. Phase conjugation of these fields at the tissue surfaces leads to the precise recovery of the initial PSF inside the tissue. Reduction of Strehl ratio was then determined as the average intensity of the focus that is recreated for laterally displaced fields at the tissue surface. The decay of focal intensity with lateral shifts were found identical to the absolute value of the spatial correlation in a speckle field that results from an incident plane-wave. The area of the isoplanatic patch was calculated as the radial integral over the gained Strehl ratio increase gained from the aberration pre-compensation. This is significantly smaller than the actual Strehl ratio only for small penetration depths (d $\leq$ 1 MFP) at which focusing still works to a residual degree without adaptive optics. For all simulations in Fig. 3c, the average of 50 different guide stars at 150 different translation position were simulated for for the shift-shift memory effect at 4 different depths, comprising 30000 PSF calculations.

# References


1. Choi, W. *et al. Nature Methods* **4** (2007).
2. Fertig, M. & Brenner, K.-H. *J. Opt. Soc. Am.* **27,** 709–717 (2010).
3. Van Roey, J., Van der Donk, J. & Lagasse, P. *J. Opt. Soc. Am.* **71,** 803–810 (1981).
4. Born, M. & Wolf, E. *Principles of Optics* 7th ed. (Cambridge University Press, 1999).
5. Judkewitz, B., Horstmeyer, R., Vellekoop, I. M., Papadopoulos, I. N. & Yang, C. *Nature physics* **11,** 684–689 (2015).
6. Jacques, S. L. *Physics in Medicine and Biology* **58,** R37 (2013).
7. Goodman, J. *Introduction to Fourier Optics* 2nd ed. (MaGraw-Hill, 1996).
8. Klöckner, A. *et al. Parallel Computing* **38,** 157–174. ISSN: 0167-8191 (2012).
9. Foreman, M. R. & Török, P. *Journal of Modern Optics* **58,** 339–364 (2011).
10. Chen, B.-C. *et al. Science* **346,** 1257998 (2014).
11. Ringler, M. *Plasmonische Nahfeldresonatoren aus zwei biokonjugierten Goldnanopartikeln* PhD thesis (LMU, 2008).
12. Oskooi, A. F. *et al. Computer Physics Communications* **181,** 687 (Mar. 2010).
13. Huisken, J., Swoger, J., Del Bene, F., Wittbrodt, J. & Stelzer, E. H. *Science* **305,** 1007–1009 (2004).
14. Nagy, J. G. & O'Leary, D. P. *SIAM Journal on Scientific Computing* **19,** 1063–1082 (1998).
15. Vellekoop, I. M. & Mosk, A. *Optics Letters* **32,** 2309–2311 (2007).
